# Supplementary material for: Improving approximate Bayesian computation via quasi-Monte Carlo
Source: arXiv:1710.01057 source file (2018-05-07)
Supplement: Supplementary file 1 [file appendix_figures.tex]

\subsection{Figures}
Here we show additional figures that are not part of the main part of the paper, but that we refer to.

%\subsubsection{Lotka-Volterra model}
%\begin{figure}[H]
%\centering
%  \includegraphics[width=0.8\linewidth]{figures/lotka_volterra_model}
%\caption{Based on 100.000 simulations and the $1\%$ quantile of the distance} 
%\label{fig:lotka_volterra_scatter}
%\end{figure}

\subsubsection{Non--sequential Gaussian toy model}
\begin{figure}[H]
\centering
\begin{subfigure}{.45\textwidth}
  \centering
  \includegraphics[width=1\linewidth]{figures/appendix/mean_mixed_gaussian_static_dim_2}
  \caption{Left}
  \label{fig:appendix_mix_gaussian_dim2}
\end{subfigure}%
\begin{subfigure}{.45\textwidth}
  \centering
  \includegraphics[width=1\linewidth]{figures/appendix/var_mixed_gaussian_static_dim_2}
  \caption{Right}
  \label{fig:appendix_mix_gaussian_dim2_var}
\end{subfigure}
\caption{Variance of the estimators for the toy model of dimension 2. Plots based on $40$ repetitions of $10^6$ simulations from the prior and the model. The accepted observations correspond to quantiles based on the smallest distances $\delta(y_n,y^*) $. Left: variance of posterior mean estimator. Right: variance of posterior variance estimator. } 
\label{fig:appendix_mix_gaussian_dim22}
\end{figure}

\begin{figure}[H]
\centering
\begin{subfigure}{.45\textwidth}
  \centering
  \includegraphics[width=1\linewidth]{figures/appendix/var_mixed_gaussian_static_dim_4}
  \caption{Left}
  \label{fig:appendix_mix_gaussian_dim4}
\end{subfigure}%
\begin{subfigure}{.45\textwidth}
  \centering
  \includegraphics[width=1\linewidth]{figures/appendix/var_mixed_gaussian_static_dim_8}
  \caption{Right}
  \label{fig:appendix_mix_gaussian_dim8}
\end{subfigure}
\caption{Variance of the mean estimator for the toy model. Plots based on $40$ repetitions of $10^6$ simulations from the prior and the model. The accepted observations correspond to quantiles based on the smallest distances $\delta(y_n,y^*) $. Left: variance of posterior mean estimator in dimension 4. Right: variance of posterior mean estimator in dimension 8.} 
\label{fig:appendix_mix_gaussian_dim48}
\end{figure}

\begin{figure}[H]
\centering
\begin{subfigure}{.45\textwidth}
  \centering
  \includegraphics[width=1\linewidth]{figures/appendix/mean_mixed_gaussian_static_dim_1_m_5}
  \caption{Left}
  \label{fig:appendix_several_m5}
\end{subfigure}%
\begin{subfigure}{.45\textwidth}
  \centering
  \includegraphics[width=1\linewidth]{figures/appendix/mean_mixed_gaussian_static_dim_1_m_20}
  \caption{Right}
  \label{fig:appendix_several_m20}
\end{subfigure}
\caption{Variance of the mean estimator for the toy model. Plots based on $40$ repetitions of $10^6$ simulations from the prior and the model. The variances correspond to observations weighted with  $ 1/M \sum_{m=1}^M \ind\left\{ \cond \right\}$. Left: variance of posterior mean estimator in dimension 1 and $M=5$ simulations from the simulator for every simulation of $\thetavec$. Right: variance of posterior mean estimator as before but with $M=20$.} 
\label{fig:appendix_several_m}
\end{figure}

%\subsubsection{Sequential Gaussian toy model}

%
%\begin{figure}[H]
%\centering
%\begin{subfigure}{.5\textwidth}
%  \centering
%  \includegraphics[width=1\linewidth]{figures/l1distance_1000N_variance_epsilon}
%  \caption{L1 distance}
%  \label{fig:sequential_l1_mixed_gaussian}
%\end{subfigure}%
%\begin{subfigure}{.5\textwidth}
%  \centering
%  \includegraphics[width=1\linewidth]{figures/ESS_1000N_variance_epsilon}
%  \caption{ESS}
%  \label{fig:sequential_ESS_mixed_gaussian}
%\end{subfigure}
%\caption{Simulation with 1.000 particles} 
%\label{fig:sequential_mixed_gaussian_2}
%\end{figure}
%
%
%\begin{figure}[H]
%\centering
%\begin{subfigure}{.5\textwidth}
%  \centering
%  \includegraphics[width=1\linewidth]{figures/l1distance_10000N_variance_epsilon}
%  \caption{L1 distance}
%  \label{fig:sequential_l1_mixed_gaussian}
%\end{subfigure}%
%\begin{subfigure}{.5\textwidth}
%  \centering
%  \includegraphics[width=1\linewidth]{figures/ESS_10000N_variance_epsilon}
%  \caption{ESS}
%  \label{fig:sequential_ESS_mixed_gaussian}
%\end{subfigure}
%\caption{Simulation with 10.000 particles} 
%\label{fig:sequential_mixed_gaussian_2}
%\end{figure}
